# Supplementary material for: SMH-Bench: Benchmarking LLM Agents for Environment-Grounded Reasoning and Action in Smart Homes
Source: arXiv:2606.01912 source file (2026-06-01)
Supplement: Supplementary file 1 [file 1_app.tex]

\section{Technical appendices and supplementary material}
Technical appendices with additional results, figures, graphs, and proofs may be submitted with the paper submission before the full submission deadline (see above). You can upload a ZIP file for videos or code, but do not upload a separate PDF file for the appendix. There is no page limit for the technical appendices. 

Note: Think of the appendix as ``optional reading'' for reviewers. The paper must be able to stand alone without the appendix; for example, adding critical experiments that support the main claims to an appendix is inappropriate.
